# Supplementary material for: Visual Tracking with Intermittent Visibility: Switched Control Design and Implementation
Source: arXiv:2411.08144 source file (2024-11-12)
Supplement: Supplementary file 1 [file sec-appendix.tex]

\section*{Appendix}
\subsection{Experiment Setup}
We have implement \vtc algorithm of  Section~\ref{sec:method} on a 
\sayan{name of drone platform} and we evaluate its performance in following various target trajectories of a second drone. 
\sayan{Best if the results can be phrased as answers to various Research Questions (RQ) and not just validation of the idea.}
of our \vtc and also validate the claim we made in Theorem~\ref{thm:hybrid_stability}. 

\subsection{Experimental Setup: Target}
%\subsubsection{The target drone} 
The target drone (Figure~\ref{fig:target_chaser_drone}) is built using a 6'' frame and has a \sayan{Mention marker?}. It uses a Raspberry Pi 3\textsuperscript{\textregistered} and a Navio2\textsuperscript{\textregistered} for onboard computations. The target drone implements a trajectory tracking controller from~\cite{pmlr-v155-sun21b} and it can follow a wide range of pre-scripted trajectories. 

\sayan{State the details of the target trajectories here?}

\subsection{Pursuer: Implementation Details}

 The pursuer drone (Figure~\ref{fig:target_chaser_drone}) is built based on Aigilicious platform from the Robotics and Perception Group at UZH~\cite{Foehn22science}. The pursuer uses an Nvidia Jetson TX2\textsuperscript{\textregistered} as the main computer, an Intel RealSense T265\textsuperscript{\textregistered} for localization, and an Arducam B0385 for target detection. The Arducam can run 100fps for 640x480 resolution images and has a viewing angle of $\theta = 70^\circ$. The \vtc runs entirely on the Jetson. 
 %TP is implemented on the chaser drone and all the computation happend on-board. 

\sayan{Say something about Vicon for ground-truth.}
The drones are operated in a $5.6m\times 5.4m\times 3m$ workspace.

% \begin{figure}
%     \centering
%     \begin{minipage}{.3\textwidth}
%       \centering
%       \includegraphics[width=.4\linewidth]{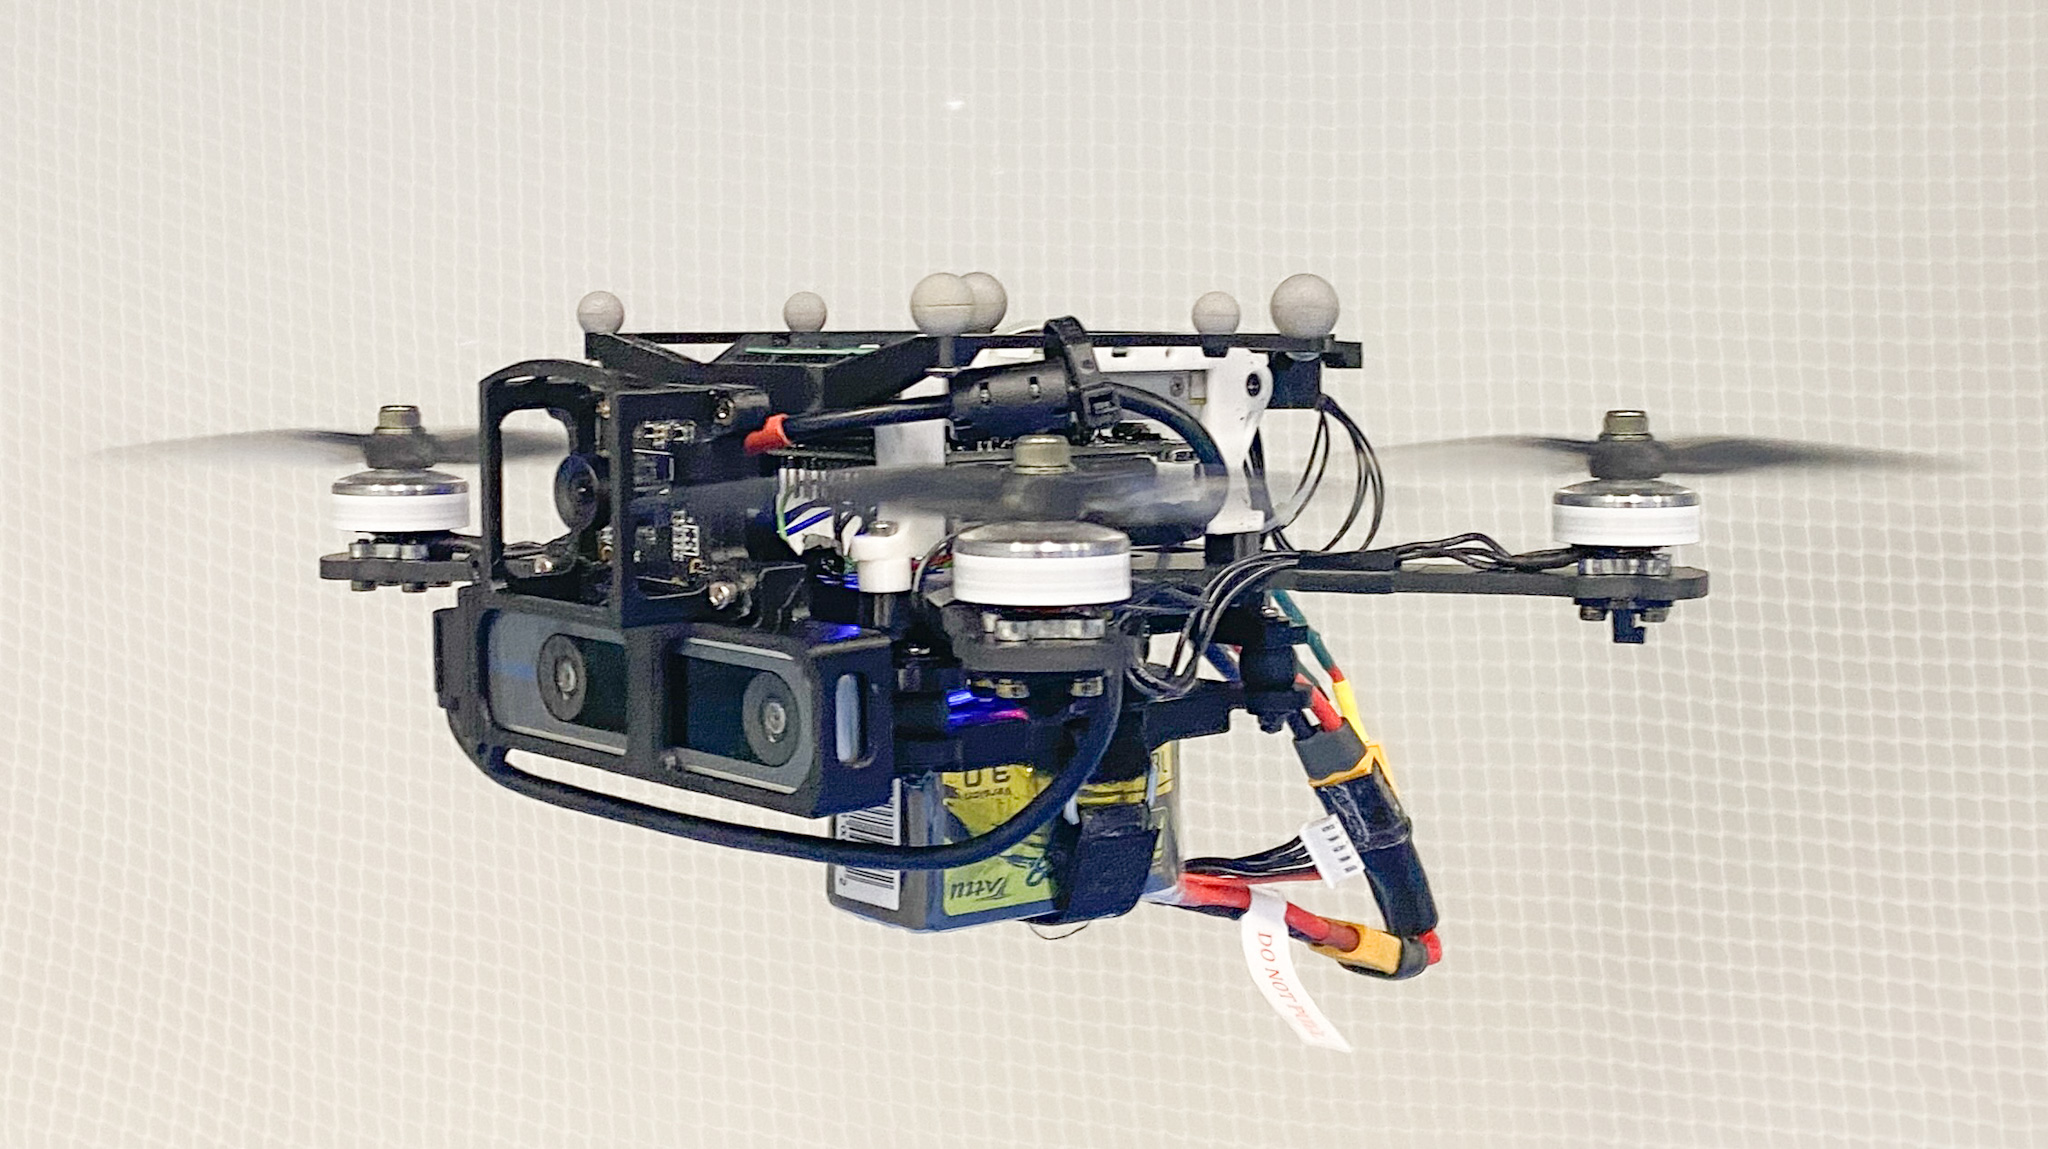}
%       \caption{Chaser Drone}
%       \label{fig:test1}
%     \end{minipage}
%     \begin{minipage}{.3\textwidth}
%       \centering
%       \includegraphics[width=.4\linewidth]{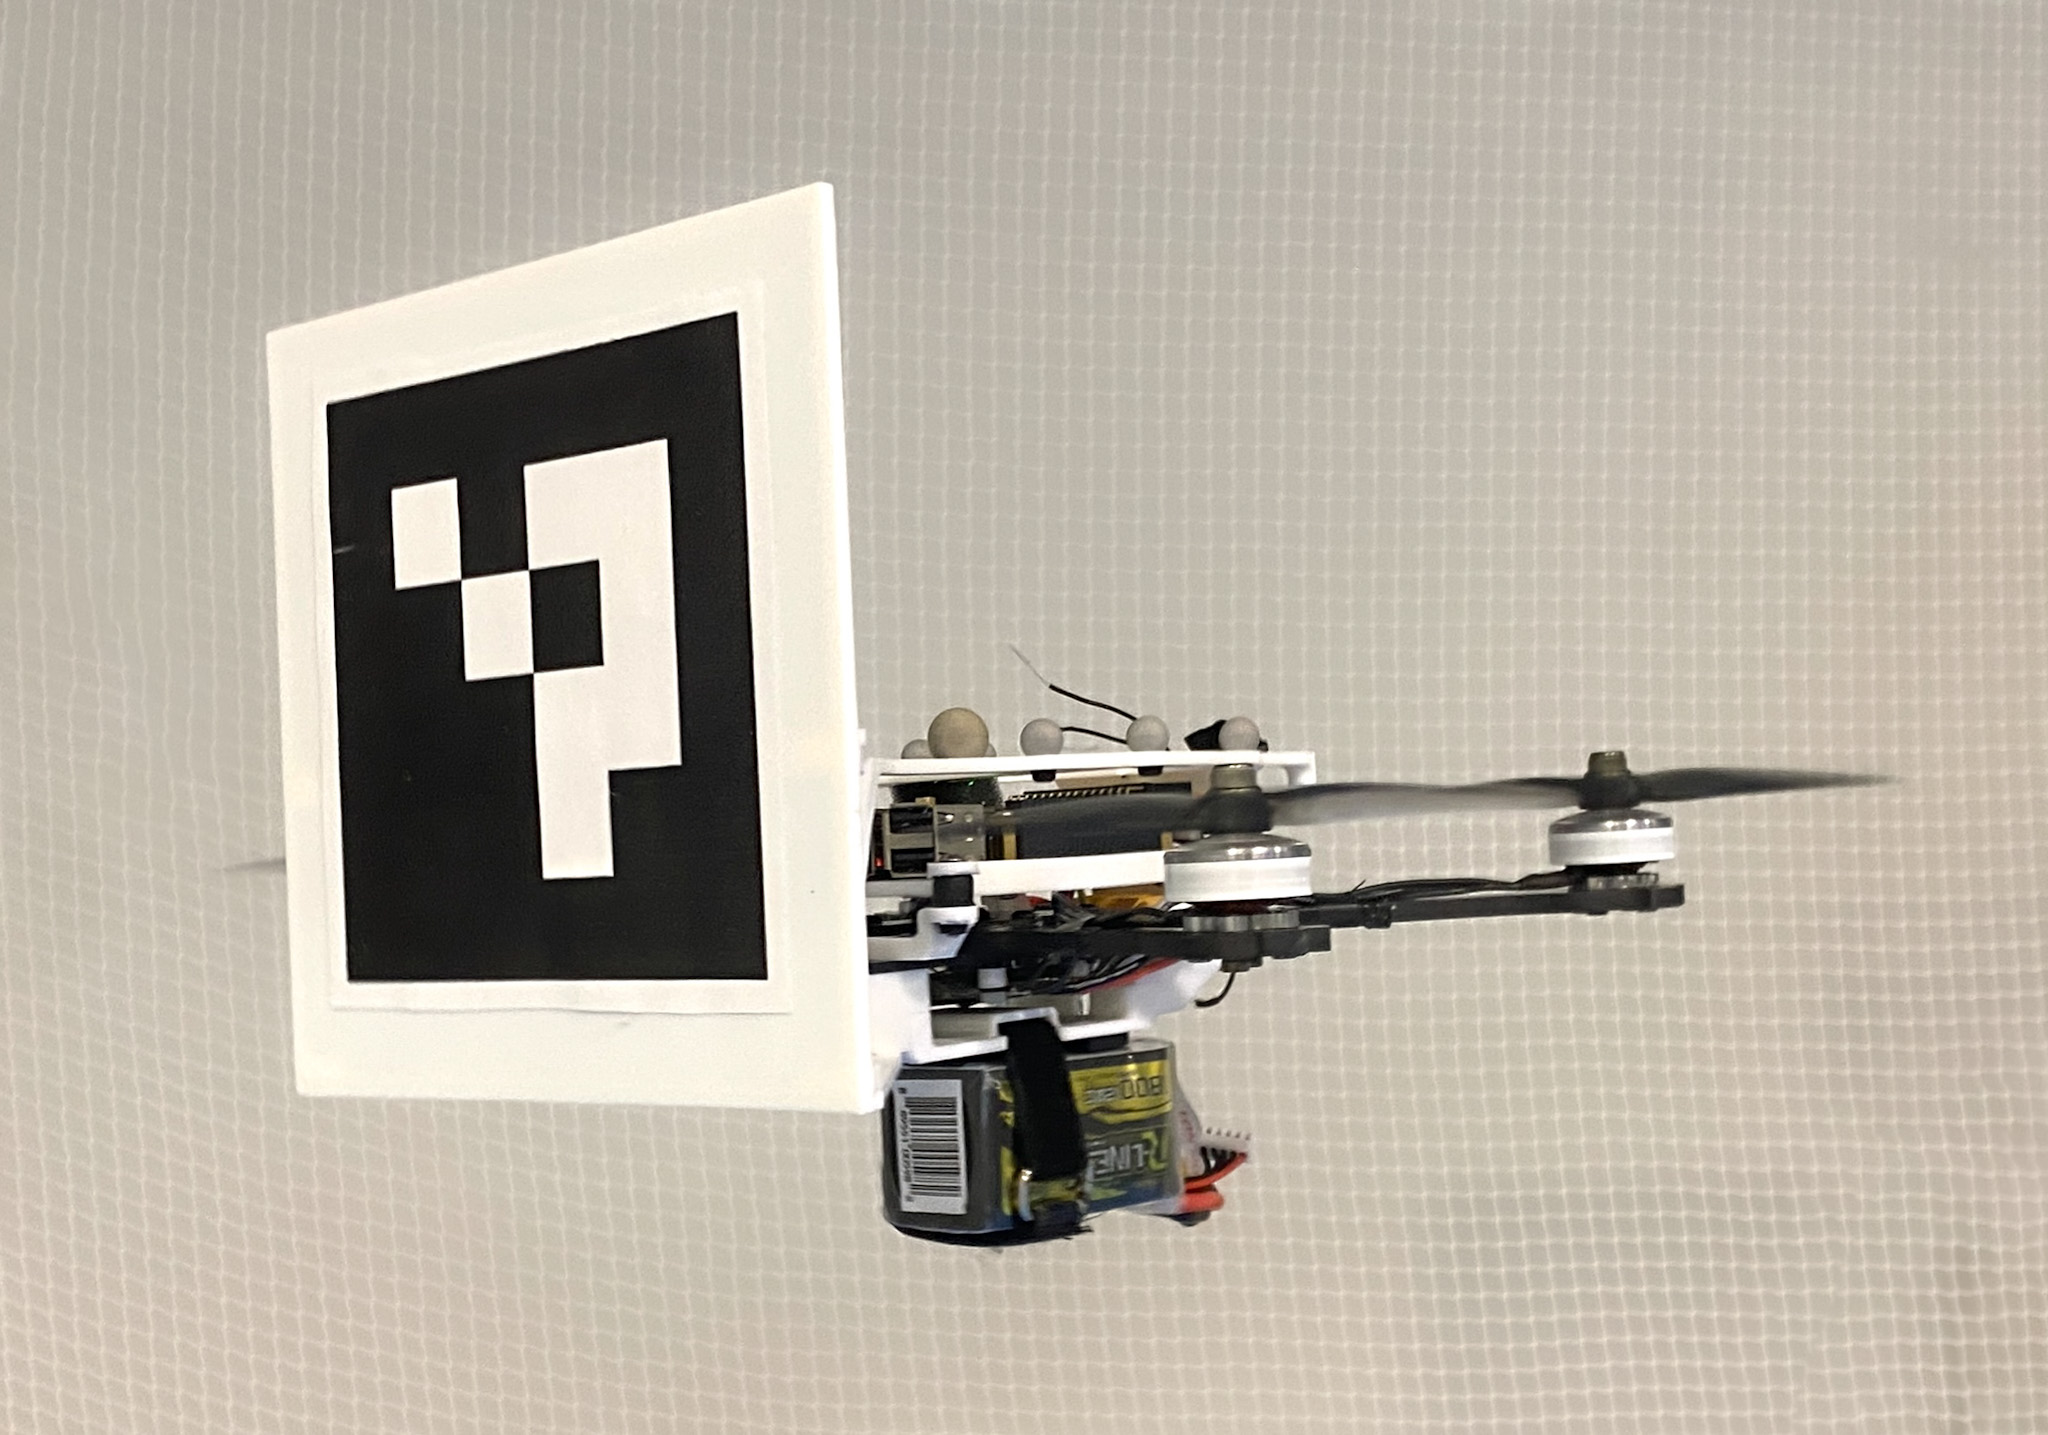}
%       \caption{Leader Drone}
%       \label{fig:test2}
%     \end{minipage}
% \end{figure}
\begin{figure}
    \centering
    \includegraphics[width=0.9\linewidth]{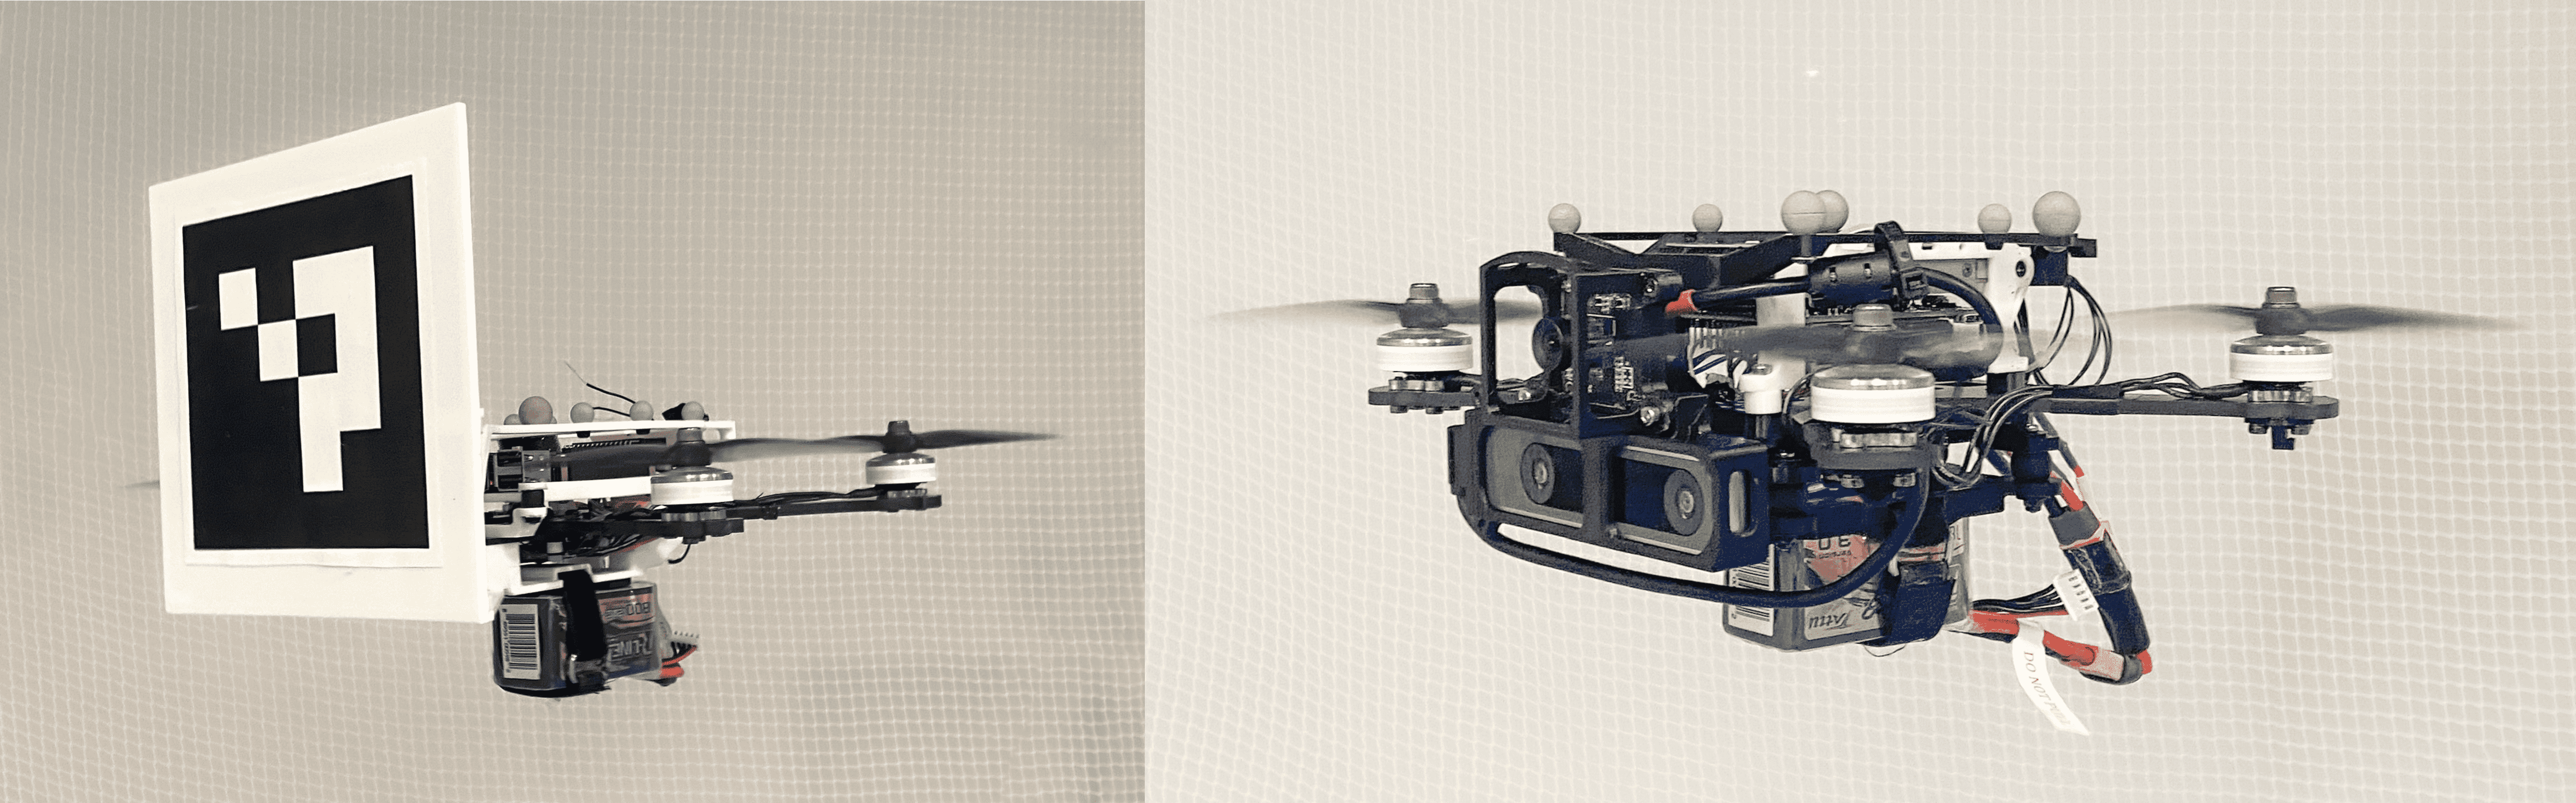}
    \caption{The target drone (left) and chaser drone (right) used in experiment}
    \label{fig:target_chaser_drone}
\end{figure}

%\subsubsection{The workspace and coordinate frame} 

\sayan{These details seem premature}
We initialize the chaser drone such that it's local frame is aligend with the world frame, i.e., positive x is moving forward, positive y is moving leftward and positive z is moving upward. The cameras on the chaser drone is pointing at positive x direction. 

\subsection{\vtc implementation details} 
The \vtc is implemented on the chaser drone. For the observer module $o$, based on our assumption in Section~\ref{sec:method:vttp_overview}, we decided to use aruco marker~\cite{}. We mount an aruco marker on the target drone and run detection algorithm~\cite{opencv_library} on images taken by the Arducam on the chaser drone to obtain accurate pose estimation of the target drone. 

A MPC controller~\cite{9794477} is used by \vtc as the tracking controller $g$ in the normal tracking mode and to drive the pursuer to the $x_R$ in the recovery mode. 

% For the low level controller $g$, we use the MPC controller implemented provided by the Agilicious drone~\cite{9794477}. 

To compute the recovery waypoint $x_R$, we assume the target follows a double integrator dynamics. The dynamics takes acceleration as input and we assume the range of acceleration between $-2m/s$ and $2m/s$.
A kalman filter is used to smooth target's position estimation and estimate its velocity. 
Reachability analysis tool Verse~\cite{10.1007/978-3-031-37706-8_18} is used to compute the forward reachable set. In this set of experiment, we assume there's no change in the yaw of both the target drone and the chaser drone. Therefore, the recovery waypoint $x_R$ is computed as 
\[
x_R = \left(c.x - \frac{r}{sin(35^\circ)},c.y, c.z\right)
\]

\subsubsection{Experiment scenarios} \sayan{With the spatial constraints in mind, we experiment with several target trajectories}  with the target is moving \sayan{parallel to the image plane of the camera}
% perpendicular to the direction of the camera, 
(which leads to frequent loss of sight).
For detailed analysis, we discuss  two target trajectories in the yz-plane with no movement in the x direction. 

\sayan{Are these details important? Maybe move to the figure caption?}
In this experiment, we design two different leader trajectories (\leadtrack) an ellipsoid (Ellip) and a square lemniscate (SLem) as shown in Fig.~\ref{fig:LTs}. The total time for Ellip is 45s, the average velocity is 0.572m/s and the maximum velocity is 0.838m/s. The total time for SLem is 40s, average velocity is 0.600 and the maximum velocity is 0.625. We let the chaser to track the leader at tracking distance 1.0m, 1.5m and 2.0m, which form 6 different experiment scenarios (\scenario) written in form \leadtrack-TD. Both trajectories are placed at the further end of the workspace, leaving enough space for the chaser to perform back-off maneuver.

\begin{figure}
    \centering
    \includegraphics[width=0.9\linewidth]{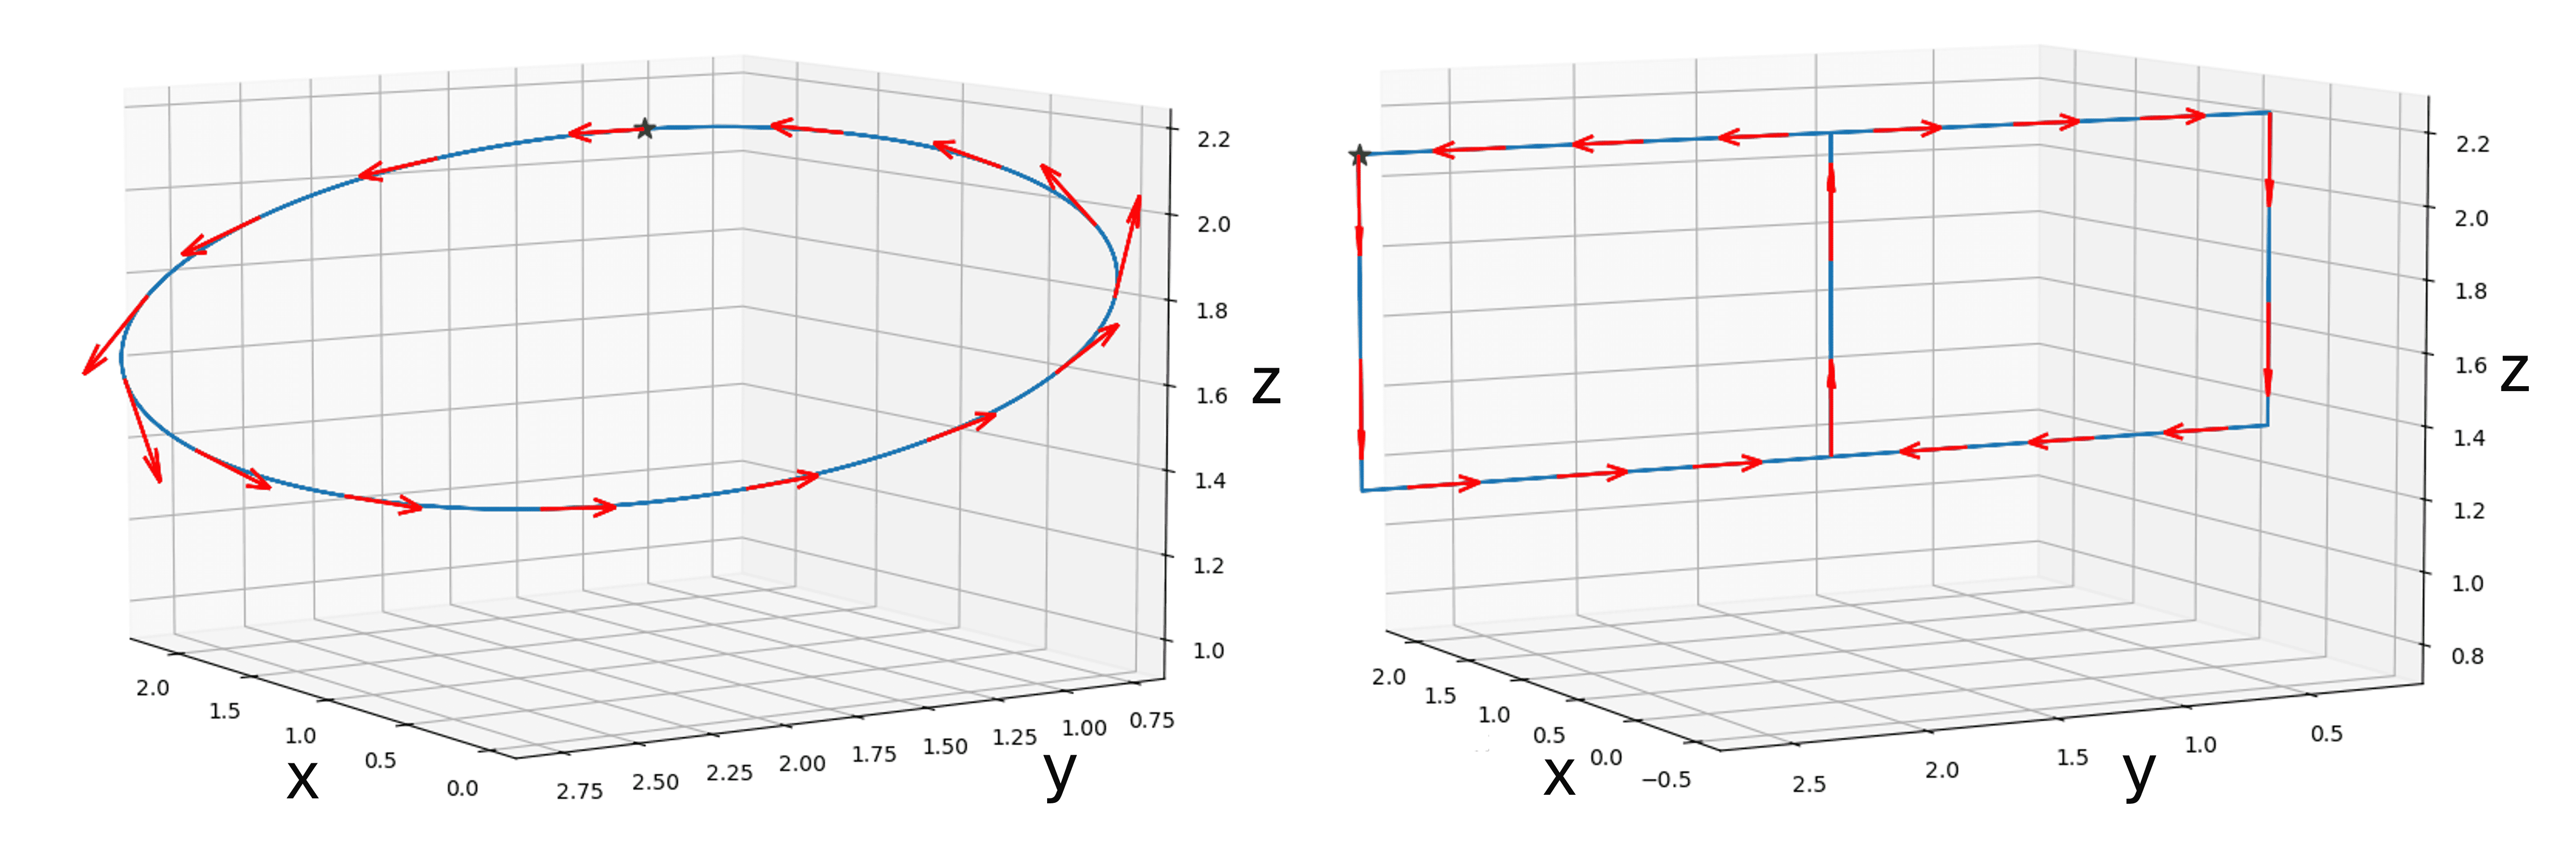}
    \caption{\small Sample of target trajectories Ellip (left) and SLem (right). \sayan{mark x,y,z coordinates clearly.} }
    \label{fig:LTs}
\end{figure}

\subsubsection{Experiment Parameters} In this experiment we mainly look at three parameters for the chaser, the maximum tracking x velocity (\maxv), the maximum back-off distance (\mbd) and the average stable dwell time (ASDT). We explore how they influence the overall tracking performance. 

\maxv limits the x velocity of the chaser in the \texttt{Normal Tracking} mode. This mainly influence how fast the chaser can move to recover from the back-off maneuver after exiting the \texttt{Recovery} mode. We uses this parameter to control the $\lambda$ in Theorem~\ref{thm:hybrid_stability}, the convergence rate of chaser's tracking controller. 

\mbd measure the maximum change in x dimension for the chaser in \texttt{Recovery} mode over each run of scenario. When letting $\mu=1$, \mbd describes $c$, the constant increase for the lyapunov function in $P\textbackslash P_s$ in Theorem~\ref{thm:hybrid_stability}. 

ASDT is one of the essential parameter in Theorem~\ref{thm:hybrid_stability} for controlling the tracking performance. We assume $N_0=1$ and ASDT is measured by 
\[
ASDT = \frac{T_s(0,T_{max})}{k-1}
\]
where k is the number of switches from \texttt{Normal Tracking} mode to \texttt{Recovery} mode in a scenario run. In this set of experiment, ASDT reflects how long chaser lose vision of target ($T_s$) and how frequent the chaser lose visual contact of target ($k$). 

Note that we don't have control over \mbd and ASDT. However, we can measure these values empirically and observe their effect on the overall tracking performance. 

\subsubsection{System Performance Metrics}
\label{exp:setup:metrics}
\sayan{We use {\em average tracking error (AE)\/}, i.e., the displacement  between the target and pursuer, and the {\em Fraction of time the target is visible (FTV)\/} from the pursuer as the two key metrics, which correspond to the proximity and the visibility requirements of the system (recall the problem definition in Section~\ref{}).}

% AE a natural metric to look at to evaluate tracking performance and is obtained by integrating the distance between the target and chaser minus the tracking distance and divide by the total time for that scenario. 

However, AE can be misleading in our experiment due to the space constraint. 
% When the chaser is position at the center of the yz plane, the maximum position difference in the yz plane is 3.1m while the maximum position difference in x direction is 5.6m. The position difference in x direction dominates 
Since for our workspace, the position error in x dimension (max 5.6m) dominates the position error in y and z (max 3.1m) dimension, it's possible that the chaser completely lose track of the target and remains stationary for the whole scenario run having better AE then one that never lose visual contact because of the smaller x error.
We further introduce the fraction of time the target is visible by the chaser (FTV) as a metric to measure the tracking performance of chaser. Note that for each leader trajectory, FTV is proportional to the total amount of time the system is in the stable mode $T_s$. According to the definition of ASDT, FTV can then roughly measure ASDT of a scenario run. 

\subsectino{Proof for Theorem~\ref{thm:hybrid_stability}}
\begin{theorem}
\label{thm:hybrid_stability}
Suppose we have a collection of Lyapunov functions $V_p$ $\forall p \in P_s$, and \yangge{there exists $\mu>1$ and $c>0$,}
such that for any switching time $t_1,t_2,...$ satisfy that $\forall i $ even, 
% \sayan{simply say any even switching times?}
\begin{equation}   
\label{eqn:v_transition_increase}
V_{\sigma(t_i)}(x(t_i))\leq \mu V_{\sigma({t_{i-1}})}(x({t_{i-1}}))+c
\end{equation}
%
% Then, for all $\delta>0 $, if the average convergence dwell time satisfy that 
Then, for any $\delta>0$, for any switching signal $\sigma$ with \sayan{ASDT} satisfy
\begin{equation}
\label{eqn:tau_a_assu}
\tau_{as} > \frac{ln(\mu+\delta)}{2\lambda}    
\end{equation}
the
the system is asymptotically stable with respect to the set 
\begin{equation}
\label{eqn:convergence_set}
    \left\{x\mid |x|\leq \alpha_1^{-1}\left(c\frac{(\mu+\delta)^{N_0}}{\delta}\right)\right\}
\end{equation}
% for every switching signal $\sigma$ the system will satisfy that as $t\rightarrow \infty$, 
% \[
% |x(T)|\leq \alpha_1^{-1}(c\frac{\mu+\delta}{\delta})
% \]
\end{theorem}

For the visual tracking problem, the state $x$ can be the state difference between the target and the pursuer, which we want it to converge to a bounded set as stated in (\ref{eqn:convergence_set}). The lyapunov function $V_p$ can be the distance between the target and pursuer. In this case, the assumption (\ref{eqn:v_transition_increase}) describe the increase of distance between target and pursuer when \vtc is in recovery mode. When the pursuer is recoverable, the recovery state $x_R$ exists and the pursuer can move the $x_R$ with in $t_R$, which indicates that the distance increase between target and pursuer in the recovery mode is upper bounded and the assumption is automatically satisfied. 

\begin{proof}
Let us fix a switching signal $\sigma:[0,\infty) \rightarrow P$.
From Equation~(\ref{eq:exp_lyapunov}), it follows that for any time interval $[t,t']$ over which there are no switches and $\sigma$ stays in a stable mode, 
\begin{equation}
\label{eqn:v_exp_decay}
V_p(x(t'))\leq V_p(x(t))e^{-2\lambda_0  (t'-t)}.  
\end{equation}
This follows from an application of Gronwall's inequality. 
Let us fix an  arbitrary time $T$, 
% \sayan{RESUME HERE.}
first consider $T$ such that $\sigma(T)\in P_s$. Consider a sequence of switching time $t_1, t_2, ..., t_N$, we can get 
\[
\begin{split}
& V_{\sigma(T)}(x(T))\\
& \leq V_{\sigma(t_N))}(x(t_N))e^{-2\lambda_0(T-t_N)} \text{~~~[Using (\ref{eqn:v_exp_decay})]}\\ 
& \leq \mu V_{\sigma(t_{N-1})}(x(t_{N-1}))e^{-2\lambda_0(T-t_N)} \\
& + c e^{-2\lambda_0(T-t_N)} \text{~~~[Using (\ref{eqn:v_transition_increase})]}\\     
\end{split}
\]

% Assume $T$ such that $\sigma(T)\in P^\da$, consider sequence of switching time $t_1, t_2, ..., t_N$, we can get 
% \[
% \begin{split}
% & V_{\sigma(T)}(x(T)) \\
% & \leq V_{\sigma(t_N))}(x(t_N))e^{-2\lambda_0(T-t_N)}\\ 
% & \leq \mu V_{\sigma(t_{N-1})}(x(t_{N-1}))e^{-2\lambda_0(T-t_N)} + c e^{-2\lambda_0(T-t_N)} \\ 
% & \leq \mu V_{\sigma (t_{N-2})}(x(t_{N-2}))e^{-2\lambda_0(T-t_N+t_{N-1}-t_{N-2})}+ce^{-2\lambda_0(T-t_N)}\\ 
% % & = \mu V_{\sigma (t_{N-2})}(x(t_{N-2}))e^{-2\lambda_0(T^\da(T, t_{N-2}))}+ce^{-2\lambda_0(T-t_N)} \\ 
% & \leq \mu^2 V_{\sigma(t_{N-3})}(x(t_{N-3}))e^{-2\lambda_0(T-t_N+t_{N-1}-t_{N-2})} + \mu c e^{-2\lambda_0(T-t_N+t_{N-1}-t_{N-2})} + ce^{-2\lambda_0(T-t_N)} \\ 
% & = \mu^2 V_{\sigma(t_{N-3})}(x(t_{N-3}))e^{-2\lambda_0T^\da(T, t_{N-2})} + \mu c e^{-2\lambda_0T^\da(T, t_{N-2})} + c e^{-2\lambda_0 T^\da(T, t_N)}
% \end{split}
% \]

If we keep unrolling the above inequliaty, we can eventually get 
\begin{equation}
\label{eqn:ineqn_unroll}
\begin{split}
& V_{\sigma(T)}(x(t)) \\
& \leq \mu^\frac{N}{2} V_{\sigma(0)}(x(0)) e^{-2\lambda_0 T_s(0,T)} + \sum_{k=0}^{\frac{N}{2}} c \mu^ke^{-2\lambda_0 T_s(t_{N-2k},T)} 
\end{split}    
\end{equation}

The right hand side of (\ref{eqn:ineqn_unroll}) is the sum of two terms, where the first term provides the transient behavior of the system and the second term provides the steady state behavior. 
\sayan{Let $V_0 = V_{\sigma(0)}x(0)$, this will make the equations below fit in one line. Maybe also shorten $T_s(0,T)$.}
Looking at the transient term in the right hand side of this inequality
\[ 
\begin{split}
& \mu^\frac{N}{2} V_{\sigma(0)}(x(0)) e^{-2\lambda_0 T_s(0,T)} \\ 
& = e^{-2\lambda_0 T_s(0,T) + ln\mu \frac{N}{2}}V_{\sigma(0)}(x(0)) 
\end{split}
\]
From definition of ASDT in (\ref{eqn:tau_a_def}), $\frac{N}{2} \leq N_0 + \frac{T_s(0,T)}{\tau_{as}}$, and from  (\ref{eqn:tau_a_assu}), we can get 
\[
\begin{split}
& exp{\left(-2\lambda_0 T_s(0,T) + ln\mu \frac{N}{2}\right)}V_{\sigma(0)}\left(x\left(0\right)\right) \\
& \leq exp{\left(-2\lambda_0 T_s(0,T) + ln\mu \left(N_0 + \frac{T_s(0,T)}{\tau_{as}}\right)\right)}\\
& ~~~~~~V_{\sigma(0)}(x(0)) \text{~~~[Using (\ref{eqn:tau_a_def})]}\\
& \leq exp{\left(-2\lambda_0 T_s(0,T) + ln\mu \left(N_0 + \frac{2\lambda_0 T_s(0,T)}{ln(\mu+\delta)}\right)\right)}\\
& ~~~~~~V_{\sigma(0)}(x(0)) \text{~~~[Using (\ref{eqn:tau_a_assu})]} \\ 
& = exp{\left(ln\mu N_0 -2\lambda_0 T_s(0,T)  \left(1-\frac{ln\mu}{ln(\mu+\delta)}\right)\right)}\\
& ~~~~~~V_{\sigma(0)}(x(0)) \\ 
& = exp{\left(-2\lambda_0 T_s(0,T)  \left(1-\frac{ln\mu}{ln(\mu+\delta)}\right)\right)}\\
& ~~~~~~\mu^{N_0}V_{\sigma(0)}(x(0))
\end{split}
\]
Since when $\mu>1$, 
\[
\frac{ln\mu}{ln(\mu+\delta)}<1
\]
as $T\rightarrow \infty$, $T_s(0,T)\rightarrow \infty$, the transient term of inequality (\ref{eqn:ineqn_unroll}) will converge to 0. 

For the steady-state term in inequality~\ref{eqn:ineqn_unroll}, since in between time interval $[t_{N-2k}, T]$, there are $k+1$ switches from unstable mode to stable modes, according to (\ref{eqn:tau_a_def}), we know $T_s(t_{N-2k},T)\geq (k+1-N_0)\tau_{as}$ for all k. Since we know $\tau_{as} \geq \frac{ln(\mu+\delta )}{2\lambda_0}$ from (\ref{eqn:tau_a_assu}), we can get 

\[
\begin{split}
& \sum_{k=0}^{\frac{N}{2}} c \mu^k \exp{\left(-2\lambda_0 T_s(t_{N-2k},T)\right)} \\
& \leq  \sum_{k=0}^{\frac{N}{2}}c \mu^k \exp{\left(-2\lambda_0(k+1-N_0)\tau_a\right)}\\
& ~~~~~ \text{~~~[Using definition of ASDT]}\\
& \leq  \sum_{k=0}^{\frac{N}{2}}c \mu^k \exp{\left(-2\lambda_0(k+1-N_0)\frac{\ln(\mu+\delta)}{2\lambda_0}\right)} \\
& ~~~~~\text{~~~[Using (\ref{eqn:tau_a_assu})]}\\ 
& = \sum_{k=0}^{\frac{N}{2}}c \mu^k \exp{\left(-(k+1-N_0) \ln(\mu+\delta)\right)}\\
& = c \sum_{k=0}^{\frac{N}{2}} \mu^k \left(\frac{1}{\exp{(\ln(\mu+\delta))}}\right)^{k+1-N_0} \\ 
& = c \sum_{k=0}^{\frac{N}{2}}\mu^k \left(\frac{1}{\mu+\delta }\right)^{k+1-N_0} \\ 
& = c (\mu+\delta)^{N_0-1}\frac{1-\left(\frac{\mu}{\mu+\delta}\right)^{\frac{N}{2}}}{1-\frac{\mu}{\mu+\delta}} \\ 
& = c\left(1-\left(\frac{\mu}{\mu+\delta}\right)^{\frac{N}{2}}\right)\frac{(\mu+\delta)^{N_0}}{\delta}
\end{split} 
\]

Since 
\[
\frac{\mu}{\mu+\delta}<1
\]
As $T$ goes to infinity, $N$ goes to infinity, the second term in right hand side of inequality~(\ref{eqn:ineqn_unroll}) will converge to a bounded constant $c\frac{(\mu+\delta)^{N_0}}{\delta}$. 

Therefore, from (\ref{eqn:v_assum1}), we can get 
\begin{equation}
\label{eqn:final_stable}
\begin{split}
|x(T)|\leq & \alpha_1^{-1}(\mu^{N_0}e^{-2\lambda_0 T_S(T,0)  (1-\frac{ln\mu}{ln(\mu+\delta)})})\alpha_2(x(0)) \\
    & + c(1-(\frac{\mu}{\mu+\delta})^{\frac{N}{2}})\frac{(\mu+\delta)^{N_0}}{\delta}    
\end{split}
\end{equation}
and as T goes to infinity, we will have 
\[
|x(T)| \leq \alpha_1^{-1}\left(c\frac{(\mu+\delta)^{N_0}}{\delta}\right)
\]

Now consider $\sigma(T)\in P\textbackslash P_s$, Consider the sequence of switching time $t_1, t_2, ..., t_N$. We know from (\ref{eqn:v_transition_increase}) that 
\[
\begin{split}
    & V_{\sigma(T)}(x(T)) \\
    & \leq \mu V_{\sigma(t_n)}(x(t_n))+c \\ 
    & \leq \mu (\mu^\frac{N-1}{2} V_{\sigma(0)}(x(0)) e^{-2\lambda_0 T_s(0,T)} \\ 
    & ~~~~~ + \sum_{k=0}^{\frac{N-1}{2}} c \mu^{k+1}e^{-2\lambda_0 T_s(T,t_{N-1-2k})} ) + c \text{~~~[Using \ref{eqn:ineqn_unroll}]} \\ 
    & = \mu^\frac{N+1}{2} V_{\sigma(0)}(x(0)) e^{-2\lambda_0 T_s(0,T)} + \sum_{k=0}^{\frac{N+1}{2}} c \mu^ke^{-2\lambda_0 T_s(t_{N-1-2k},T)}
\end{split}
\]

The rest of the proof will remain the same.  
\end{proof}
